# Supplementary material for: Sell More, Play Less: Benchmarking LLM Realistic Selling Skill
Source: arXiv:2604.07054 source file (2026-08-26)
Supplement: Supplementary file 1 [file appendix.tex]

% =============================================================================

\section{User-Model Evaluation Details}
\label{app:user-eval}

This section details the automatic evaluation protocol for the user simulator described in \cref{exp:ablation_user}.

\subsection{Evaluation Methodology}
\paragraph{User Likeness (Turn-Level Similarity).}
We evaluate the user model by predicting customer turns conditioned on ground-truth history from crowd worker dialogues. Given a dialogue context (system message + previous turns), we generate the next customer utterance and compute its similarity to the human ground truth using BLEU-4, ROUGE-1/2/L, and embedding cosine similarity (via `bge-m3'). We apply language-specific tokenization and exclude short acknowledgments (length $\le$ 5 chars) from evaluation to ensure meaningful comparison. 
\begin{table}[ht]
\small
    \centering
    \begin{tabular}{cccc}
        \toprule
         \textbf{Product}& \# \textbf{Dialogues} & \textbf{Avg. Turns} & \textbf{Avg. Msg Len} \\
         \midrule
         Security& 189 & 3.32 & 14.07 \\
         Banking & 50 & 4.79 & 10.2 \\
         Fund & 29 & 2.61 & 16.23 \\
         \bottomrule
    \end{tabular}
    \caption{The statical information of CustomerLM test data. \# Dialogues is the number of dialogues, Avg. Turns is the average turns of the dialogues, Avg. Msg Len is the average user message lengths.}
    \label{tab:user_test_data}
\end{table}

\begin{table}[t]
\centering
\small
\begin{tabular}{lrrr}
\toprule
\textbf{Lang} & \textbf{\#Dia} & \textbf{Avg msgs/conv} & \textbf{Avg user msgs} \\
\midrule
ZH (118\_zh) & 118 & 7.98 & 3.85 \\
EN (150\_en) & 150 & 8.13 & 3.83 \\
\bottomrule
\end{tabular}
\caption{Held-out ablation test set statistics (Sec.~\ref{exp:ablation_user}). Averages exclude the system prompt. Lang is language, Dia is dialogues.}
\label{tab:ablation_test_stats}
\end{table}

Below are the system prompt used with CustomerLM as the user model, along with one example of test data.

\begin{center}
\begin{promptbox}{System Prompt}
\textbf{Your task}:\\
You are a customer management expert, and you need to refer to the following content for communication and response.The customer is a customer service representative from xx Securities, a company formerly known as xx Securities. They are promoting a special offer for existing customers, which provides a stable annual return of 0.035. Specifically, an investment of 50,000 yuan over three years can yield a return of 5,250 yuan, with funds supervised by a bank to ensure safety. The customer also suggests adding the company's WeChat account for more information and assistance.

\textbf{Rules}: \\
-Use English strictly for the conversation. \\
-Be realistic and rational; do not mention things that are impossible. \\
-Avoid discussing personal life or other topics unrelated to your purchase intention. \\
-Use conversational language instead of formal writing; keep each response brief.\\
-Do not fabricate product facts; respond from a customer perspective based on your understanding.\\
-Avoid using parentheses to describe your actions or inner thoughts; just speak naturally. \\
\end{promptbox}
\end{center}

\begin{center}
\begin{promptbox}{One example of test data}
\textbf{assistant}: Hi. \\
\textbf{user}: Hello, I am a customer service representative from xx Securities. Our company's previous name was xx Securities, do you remember? \\
\textbf{assistant}: What? \\
\textbf{user}: The company formerly known as xx Securities has now been renamed to xx Securities. I remember you have used our services before, right? \\
\textbf{assistant}: Oh, I remember now. \\
\textbf{user}: That's correct, the original XX Securities is now called XX Securities. We are reaching out to you today because there is a special promotional event for our long-time clients, where you can receive a stable annual return of 0.035. May I provide you with more details? \\
\textbf{assistant}: Okay, please tell me the details. \\
\textbf{user}: Of course. This activity is very simple: you just need to join with your idle funds and become our esteemed member to receive corresponding returns. For example, if you invest 50,000 yuan for three years, you can receive a total return of 5,250 yuan, with an annualized return rate of 0.035. These returns can be directly transferred to your bank account. Additionally, the funds are regulated by the bank to ensure the safety of your principal. Does this explanation help you understand? \\
\textbf{assistant}: I understand, but I still have some concerns about security. \\
\textbf{user}: Rest assured, your funds will be deposited in your personal bank account and monitored by the bank. It's like a margin, providing you with membership privileges and vehicle insurance protection through our platform. \\
\textbf{assistant}: Okay.\\
\textbf{user}: If this activity interests you, you can open WeChat and follow our official account. Are you able to use WeChat now? You can start by adding our corporate WeChat account. \\
\textbf{assistant}: I don't have time right now, but I have already learned some information. \\

\end{promptbox}
\end{center}
\paragraph{Role Inversion (Conversation-Level Consistency).}
Role inversion occurs when the user model incorrectly adopts the salesperson's role (e.g., pitching features). We detect this using a GPT-4o-based judge with the prompt in Prompt~\ref{prompt:role-inversion}. For the ablation study, we sample 100 scenarios from the benchmark and generate dialogues using each user model variant (CustomerLM, GPT-4o, UserLM, USP) against three diverse sales agents: Gemini-3-Flash, Llama-3.3-70B, and GPT-5-Nano. The GPT-4o judge evaluates every generated user turn for role-reversal behavior. The Role Inversion Rate is calculated as the ratio of turns flagged as "role inversion" to the total number of user turns generated across all conversations: $\text{Rate} = \frac{\sum \text{Flagged Turns}}{\sum \text{Total Turns}}$.

\begin{center}
\begin{promptbox}{Prompt: Role Inversion Detector}
\label{prompt:role-inversion}
\small
Please analyze the following sales conversation and determine if the USER incorrectly acted as the ASSISTANT.

\textbf{Conversation:}
\{conversation\_text\}

\textbf{Your Task:}
Check the USER's messages to see if they exhibited "Role Reversal" (i.e., the USER started pitching products, offering services, or acting like a customer service agent/salesperson).

\textbf{Criteria:}
1. \textbf{Role Reversal}: The USER proactively explains product features, offers quotes, appeases the customer, or asks "How can I help you?" - behaviors clearly belonging to a sales/support role.
2. \textbf{Normal Interaction}: The USER asks questions, states needs, bargains, refuses, or accepts. These are normal USER behaviors.

Please output JSON in this format:
\{
    "detected": true/false,
    "severity": "none/low/medium/high",
    "reason": "Brief reason for judgment",
    "examples": ["Incorrect statement by USER 1", "Incorrect statement by USER 2"]
\}

\textbf{Note:}
- Set 'detected' to true if ANY obvious sales/support behavior is found in USER messages.
- Output ONLY JSON. Do not include Markdown formatting or other text.
\end{promptbox}
\end{center}

\subsection{Results}
Table~\ref{tab:user_likeness_stats} presents turn-level statistics on the held-out test set (268 dialogues). Our CustomerLM consistently outperforms the GPT-4o baseline across lexical and semantic metrics.

\begin{table}[t]
\centering
\small
\begin{tabular}{lcc}
\toprule
\textbf{Metric} & \textbf{GPT-4o} & \textbf{CustomerLM} \\
\midrule
N evaluated turns & 750 & 751 \\
History length & 5.33 & 5.33 \\
BLEU-4 & 0.1000 $\pm$ 0.1635 & \textbf{0.1218} $\pm$ 0.1749 \\
ROUGE-1 & 0.0846 $\pm$ 0.1207 & \textbf{0.1062} $\pm$ 0.1499 \\
ROUGE-2 & 0.0176 $\pm$ 0.0554 & \textbf{0.0250} $\pm$ 0.0790 \\
ROUGE-L & 0.0725 $\pm$ 0.1064 & \textbf{0.0985} $\pm$ 0.1414 \\
Embedding cosine & 0.5682 $\pm$ 0.1182 & \textbf{0.5922} $\pm$ 0.1266 \\
\bottomrule
\end{tabular}
\caption{Turn-level user-likeness statistics on the held-out set (mean $\pm$ std; without “±”: mean). Best results are bolded.}
\label{tab:user_likeness_stats}
\end{table}

\begin{comment}
\subsection{Dialogue Turn Analysis}
\label{app:dialogue_turns}

Figure~\ref{fig:score} analyzes the correlation between SalesLLM scores and dialogue lengths.

\begin{figure}[htbp]
    \centering
    \begin{minipage}{0.8\linewidth}
        \centering
        \includegraphics[width=\linewidth]{figs/legend_score.png}
    \end{minipage}
    \vspace{0.5em}

    \begin{subfigure}{0.95\linewidth}
        \centering
        \includegraphics[width=\linewidth]{figs/score.png}
        \caption{GPT-4o User Model}
        \label{fig:score-a}
    \end{subfigure}
    \hfill
    \vspace{0.3em}
    \begin{subfigure}{0.95\linewidth}
        \centering
        \includegraphics[width=\linewidth]{figs/score_cus.png}
        \caption{SalesLLM Custom User Model}
        \label{fig:score-b}
    \end{subfigure}

    \caption{Distribution of SalesLLM scores vs. dialogue turns across 1,805 scenarios (Chinese and English).}
    \label{fig:score}
\end{figure}
\end{comment}
\section{Scenario and Persona Statistics}
\label{app:scenario-persona}

SalesLLM leverages a structured scenario space combining diverse product catalogs and personas.

\subsection{Scenario Space Overview}
\label{app:scenario-stats}
\label{app:scenario-generation}

Table~\ref{tab:scenario-stats} summarizes the scale of our scenario components. We synthesized 10,074 E-commerce items from 33 seed categories (Table~\ref{tab:category-dist}) and 20,000 financial services products (Table~\ref{tab:finance-category-dist}) from 300 seeds.

\begin{table}[t]
\centering
\small
\begin{tabular}{lrr}
\toprule
Component             & \# Seeds & \# Instances \\
\midrule
E-commerce products & 33      & 10{,}074    \\
Financial services    & 300     & 20{,}000    \\
User personas         & --      & 19{,}138    \\
\bottomrule
\end{tabular}
\caption{Statistics of the SalesLLM scenario space.}
\label{tab:scenario-stats}
\end{table}

\begin{table}[t] 
 \centering 
 \small 
 \begin{tabular}{p{0.49\linewidth}rr} 
 \toprule 
 Category & \#instances & Share (\%) \\ 
 \midrule 
 \texttt{\detokenize{Pet_Supplies}} & 392 & 3.89 \\ 
 \texttt{\detokenize{Magazine_Subscriptions}} & 367 & 3.64 \\ 
 \texttt{\detokenize{Patio_Lawn_and_Garden}} & 364 & 3.61 \\ 
 \texttt{\detokenize{Office_Products}} & 361 & 3.58 \\ 
 \texttt{\detokenize{Health_and_Personal_Care}} & 358 & 3.55 \\ 
 \texttt{\detokenize{Sports_and_Outdoors}} & 351 & 3.48 \\ 
 \texttt{\detokenize{Gift_Cards}} & 351 & 3.48 \\ 
 \texttt{\detokenize{Grocery_and_Gourmet_Food}} & 346 & 3.43 \\ 
 \texttt{\detokenize{Clothing_Shoes_and_Jewelry}} & 341 & 3.38 \\ 
 \texttt{\detokenize{Beauty_and_Personal_Care}} & 330 & 3.28 \\ 
 \texttt{\detokenize{Automotive}} & 322 & 3.20 \\ 
 \texttt{\detokenize{Handmade_Products}} & 321 & 3.19 \\ 
 \texttt{\detokenize{Tools_and_Home_Improvement}} & 321 & 3.19 \\ 
 \texttt{\detokenize{Amazon_Fashion}} & 319 & 3.17 \\ 
 \texttt{\detokenize{Toys_and_Games}} & 317 & 3.15 \\ 
 \texttt{\detokenize{Industrial_and_Scientific}} & 313 & 3.11 \\ 
 \texttt{\detokenize{CDs_and_Vinyl}} & 301 & 2.99 \\ 
 \texttt{\detokenize{Home_and_Kitchen}} & 298 & 2.96 \\ 
 \texttt{\detokenize{Health_and_Household}} & 296 & 2.94 \\ 
 \texttt{\detokenize{Cell_Phones_and_Accessories}} & 296 & 2.94 \\ 
 \texttt{\detokenize{Baby_Products}} & 291 & 2.89 \\ 
 \texttt{\detokenize{Musical_Instruments}} & 284 & 2.82 \\ 
 \texttt{\detokenize{Video_Games}} & 279 & 2.77 \\ 
 \texttt{\detokenize{Subscription_Boxes}} & 271 & 2.69 \\ 
 \texttt{\detokenize{Books}} & 271 & 2.69 \\ 
 \texttt{\detokenize{Digital_Music}} & 270 & 2.68 \\ 
 \texttt{\detokenize{Arts_Crafts_and_Sewing}} & 268 & 2.66 \\ 
 \texttt{\detokenize{Kindle_Store}} & 266 & 2.64 \\ 
 \texttt{\detokenize{Software}} & 260 & 2.58 \\ 
 \texttt{\detokenize{All_Beauty}} & 251 & 2.49 \\ 
 \texttt{\detokenize{Electronics}} & 235 & 2.33 \\ 
 \texttt{\detokenize{Movies_and_TV}} & 232 & 2.30 \\ 
 \texttt{\detokenize{Appliances}} & 231 & 2.29 \\ 
 \midrule 
 \textbf{Total} & \textbf{10{,}074} & \textbf{100.00} \\ 
 \bottomrule 
 \end{tabular} 
 \caption{Category distribution of the E-commerce scenario space in SalesLLM.} 
 \label{tab:category-dist} 
 \end{table}

\begin{table}[t]
\centering
\small
\begin{tabular}{lrr}
\toprule
Category & \# Instances & Share (\%) \\
\midrule
\texttt{bank\_deposits} & 10{,}521 & 52.61 \\
\texttt{stocks}        & 6{,}109  & 30.55 \\
\texttt{insurance}     & 2{,}858  & 14.29 \\
\texttt{bund\_fund}     & 512      &  2.56 \\
\midrule
\textbf{Total} & \textbf{20{,}000} & \textbf{100.00} \\
\bottomrule
\end{tabular}
\caption{Distribution of Financial Services categories.}
\label{tab:finance-category-dist}
\end{table}

\subsection{Decision-Factor Taxonomy}
\label{app:decision-factor-taxonomy}
% We categorize user decision factors into ten dimensions, including \textit{Returns \& Cost}, \textit{Safety}, \textit{Brand Trust}, and \textit{Convenience}, to enable structured preference modeling:
We categorize user decision factors into ten dimensions to enable structured preference modeling:
\begingroup
\small
\setlength{\parindent}{0pt}
\setlength{\parskip}{0.15em}

\newcommand{\dfcat}[2]{%
  \paragraph{#1}\hspace{0.25em}#2%
}

\dfcat{Returns \& Total Cost}{%
How much value the user gets for the money: yield, interest, or returns versus
all costs such as fees, premiums, deductibles, and potential hidden charges.}

\dfcat{Safety \& Protection}{%
How safe the money or product is: insurance or guarantees (e.g., FDIC),
security controls, safety certifications, fraud protection, and overall risk
containment.}

\dfcat{Brand Trust \& Institutional Stability}{%
Whether the provider feels reliable in the long term: reputation, track record,
financial stability, and confidence that it will not fail or cause problems later.}

\dfcat{Core Quality / Fundamental Strength}{%
The underlying “real” strength of what is being bought: product build and
performance, service reliability, or (for investments) business fundamentals
and earnings quality.}

\dfcat{Transparency \& Terms Clarity}{%
How clear and honest the information is: understandable terms and policies,
simple pricing, clear disclosures, and a low chance of unpleasant surprises.}

\dfcat{Support, Claims \& After-Sales}{%
What happens after purchase: customer service quality, claims and returns
handling, issue resolution speed, and how painless the overall support process feels.}

\dfcat{Convenience \& Digital Experience}{%
How easy the product or service is to use day-to-day: mobile app quality,
online workflows, speed of setup, and overall user experience with minimal friction.}

\dfcat{Availability \& Delivery Speed}{%
How fast and reliably the user can get access: shipping speed, installation
timing, access to funds, and general availability when needed.}

\dfcat{Social Proof \& Third-Party Validation}{%
External signals that reduce uncertainty: customer reviews, peer
recommendations, expert ratings, analyst opinions, and trusted media or creators.}

\dfcat{Fit \& Flexibility}{%
How well the option matches the user’s personal situation and how adaptable it is:
customization, coverage fit, liquidity or withdrawal flexibility, and handling of edge cases.}

\endgroup

\begin{comment}
\subsection{Difficulty Control}
\label{app:difficulty-control}
Scenarios are assigned one of five difficulty profiles (\emph{easy} to \emph{adversarial}) controlling buy propensity ($p_k$) and decision timing ($t_{\text{dec}}$). A stochastic policy determines the final outcome based on the agent's performance within the allowed decision window.
\end{comment}

\section{Example Scenarios}
\label{app:example-scenarios}

We provide representative examples of instantiated scenarios below. Each scenario includes the product information, customer persona, and an excerpt from the dialogue script.

\subsection{Financial Services: Bank Deposit}
\textbf{Product}: High-Yield Fixed Deposit (Tiered Rate)
\begin{itemize}
    \item \textbf{Type}: Fixed-term Deposit (R1 Low Risk)
    \item \textbf{Interest Rates}:
    \begin{itemize}
        \item 1-Year Term: 3.0\%
        \item 2-Year Term: 3.5\%
        \item 3-Year Term: 4.0\%
    \end{itemize}
    \item \textbf{Minimum Deposit}: 50,000 RMB
    \item \textbf{Key Features}:
    \begin{itemize}
        \item Principal and interest fully guaranteed up to 500,000 RMB (Deposit Insurance).
        \item Supports early withdrawal (including partial withdrawal) for liquidity needs.
        \item Interest rates significantly higher than the benchmark rate.
    \end{itemize}
\end{itemize}

\textbf{Customer Persona}
\begin{itemize}
    \item \textbf{Profile}: 45-55yo Male, Mechanical Engineer, based in Luoyang.
    \item \textbf{Motivations}: Primary goal is to ensure retirement safety and reserve funds for children's education. Seeks stable returns through regular deposits.
    \item \textbf{Pain Points}: Deeply concerned about the low interest rates of current bank deposits and the uncertainty of the economic environment. Worries about insufficient liquidity if funds are locked up.
    \item \textbf{Decision Factors}: Prioritizes high interest rates, flexibility of deposit terms (to manage liquidity), bank reputation, and deposit insurance coverage.
    \item \textbf{Communication Preferences}: Trusts traditional media and acquaintance recommendations. Prefers clear information via bank branches or phone consultations.
    \item \textbf{Behavior (Easy Profile)}: Open and proactive buyer with a buy-inclination score of 0.8. Has a flexible budget and clear needs. If the product matches his requirements (high rate + safety), he is inclined to make quick decisions with minimal resistance.
\end{itemize}

\textbf{Dialogue Snippet}
\begin{quote}
\small
\textbf{Assistant}: "I understand your need for stable returns and liquidity. Our High-Yield Savings offers tiered rates up to 4.0\% for a 3-year term, which is significantly above the benchmark. Plus, it supports partial early withdrawal, so you can access funds if needed without breaking the entire deposit."\\
\textbf{User}: "That 4.0\% rate sounds attractive for my retirement savings. Is the principal guaranteed?"\\
\textbf{Assistant}: "Yes, absolutely. Your principal and interest up to 500,000 are fully protected by deposit insurance, ensuring your retirement funds are safe regardless of market fluctuations."
\end{quote}

\subsection{Consumer Goods: Vacuum Cleaner}
\textbf{Product}: Dyson V11 Animal Cordless Stick Vacuum
\begin{itemize}
    \item \textbf{Category}: Appliances > Vacuum Cleaners
    \item \textbf{Key Features}: 60-minute battery life, 185 AW suction, HEPA filter, convertible to handheld.
    \item \textbf{Price}: Premium range.
\end{itemize}

\textbf{Customer Persona}
\begin{itemize}
    \item \textbf{Profile}: 30-40yo pet owner, Apartment dweller.
    \item \textbf{Motivations}: Needs efficient cleaning for pet hair; values convenience.
    \item \textbf{Pain Points}: Current vacuum is heavy and corded; doesn't pick up cat hair well.
    \item \textbf{Behavior}: Pragmatic, looks for efficiency and ease of use.
\end{itemize}

\textbf{Dialogue Snippet}
\begin{quote}
\small
\textbf{Assistant}: "The Dyson V11 is specifically engineered for homes with pets. Its high-torque cleaner head automatically adapts suction power to deep clean carpets and remove stubborn pet hair."\\
\textbf{User}: "Does the battery really last long enough for a whole apartment?"\\
\textbf{Assistant}: "Yes, it offers up to 60 minutes of fade-free power, which is typically more than enough for a standard apartment. plus, the LCD screen shows you the remaining run time in real-time."
\end{quote}

\section{BERT vs. GPT-4o Classifier}
\label{app:bert-confusion}
We validate our fine-tuned BERT classifier against GPT-4o (LLM-as-a-Judge). Table~\ref{tab:bert-comparison} shows that our specialized model achieves significantly higher accuracy (>$90\%$) compared to GPT-4o ($68-74\%$) for buying intention detection.

\begin{table}[h]
\centering
\small
\begin{tabular}{lcccc}
\toprule
\textbf{Model} & \textbf{Lang} & \textbf{Acc} & \textbf{F1} \\
\midrule
GPT-4o & ZH & 69.6\% & 0.73 \\
Trained BERT & ZH & \textbf{93.51\%} & \textbf{0.93} \\
\midrule
GPT-4o & EN & 68.85\% & 0.72 \\
Trained BERT & EN & \textbf{92.94\%} & \textbf{0.93} \\
\bottomrule
\end{tabular}
\caption{Accuracy comparison: Fine-tuned BERT vs. GPT-4o. Lang is language (ZH is Chinese, EN is English), Acc is accuracy and F1 is F1 score.}
\label{tab:bert-comparison}
\end{table}

\section{Script Examples}
\label{app:sc_example}
%This appendix provides the core prompt templates used in SalesLLM to instantiate the sales agent and evaluate performance.
Example of a customer script and a salesperson script.
%\subsection{Customer Scripts Example}
%\label{app:sc}
\begin{center}
\begin{promptbox}{User Script Example}
\label{prompt:customer}
\footnotesize
- Difficulty level: medium  \\
- Buy-inclination score: 0.6  \\
- Persona: Balanced buyer. Has some concerns (price/fit) and needs reasonable evidence. Will buy if key objections are addressed satisfactorily. Inclined to purchase, but will raise reasonable questions and concerns. If they are confident enough about the product and these issues are resolved satisfactorily, they may buy.\\  

- CUSTOMER\_INFORMATION (private to you):\\  
  - basic\_info: {"age\_group": "45-55", "gender": "male", "location": "Shanghai", "occupation": "senior business consultant"}  \\
  - motivations: Hopes to subscribe to a professional technology magazine to obtain cutting-edge technical insights, innovation trends, and cultural dynamics to assist their business consulting work and fulfill their interest in the technology field.\\  
  - pain\_points: Has doubts about product quality authenticity, worries about inadequate after-sales service and payment security issues; at the same time hopes that the subscription magazine’s content is professionally detailed and has good brand credibility.  \\
  - decision\_factors: Values brand credibility, product reviews, after-sales guarantees, payment security, and logistics speed; also pays attention to the professionalism, depth, and uniqueness of the magazine content.  \\
  - communication\_preferences: Prefers WeChat and email; likes formal, professional, detailed content with text and images.\\  
  - language: english\\
\end{promptbox}
\end{center}

%\subsection{Salesman Script Example}
\begin{center}
\begin{promptbox}{Salesperson Script Example}
\label{prompt:sales}
\footnotesize

You are a professional salesperson (ASSISTANT) in a realistic sales conversation.\\
Only you can see the following PRODUCT\_INFORMATION. Never reveal it or where it came from. Speak naturally and be helpful.\\

You should use sales strategies and techniques to persuade the customer. If the customer has committed to buying the product, you should provide a purchase channel if it is available in PRODUCT\_INFORMATION. 
else, you should provide a reason why the customer should buy the product.\\

PRODUCT\_INFORMATION (private to you):\\
main\_category: Magazine Subscriptions\\
title: Wired Magazine Subscription - 12 Issues/Year - Print Only - Cutting-Edge Tech, Innovation, and Cultural Trends\\
price: \$39.99/Year\\
store: TechMagStore\\
categories:\\
  Magazine Subscriptions\\
  Technology\\
  Computers \& Electronics\\
details:\\
  Subscription Type: Print Only\\
  Frequency: Monthly\\
  Number of Issues: 12\\
  Publisher: Condé Nast\\
  Item model number: WIRED-MS-12P\\
  Best Sellers Rank: {'Magazine Subscriptions': 289, 'Technology Magazines': 11}\\
  Date First Available: January 10, 2020\\
  Brand: Wired\\
  Format: Print\\
  Shipping Weight: 0.7 pounds per issue\\
  Cover Art: Exclusive artist collaborations monthly\\
  Included Bonus: Free The Wired Guide to AI digital download\\
\texttt{[}12 MONTHLY ISSUES OF TECH INSIGHT\texttt{]}: Dive into the future of technology with 12 monthly issues packed with in-depth features on AI, cybersecurity, space travel, and the intersection of tech and culture—written by Wired’s award-winning journalists and industry insiders.\\
  \texttt{[}PRINT-ONLY COLLECTOR’S EDITION\texttt{]}: Our print issues feature high-quality matte paper, exclusive cover art from renowned tech artists, and fold-out infographics that make complex topics like quantum computing easy to understand—perfect for tech enthusiasts who love physical media.\\
  \texttt{[}BEHIND-THE-SCENES CONTENT\texttt{]}: Each issue includes a "Tech Makers" section profiling engineers building the next big thing, plus a "Gadget Lab" with hands-on reviews of the latest smartphones, laptops, and smart home devices.\\
  \texttt{[}SUBSCRIBER-ONLY EVENTS\texttt{]}: Get invited to virtual Q\&As with Wired editors, early access to our annual "Wired 25" list of top innovators, and a free digital copy of "The Wired Guide to AI" to stay ahead of tech trends.\\
  \texttt{[}RISK-FREE SUBSCRIPTION\texttt{]}: We stand behind our content—if you’re not satisfied with your first 3 issues, we’ll give you a full refund. No hidden fees, no automatic renewals without notice!\\

Rules:\\
- Speak strictly in English.\\
- Be professional and helpful. Do not chat your personal life or anything unrelated to the product.\\
- Do not speak too many words in one turn, keep your replies concise and realistic.\\
- Be friendly and engaging.\\
- Do not leak or quote the PRODUCT\_INFORMATION verbatim.\\
- Base your answers on PRODUCT\_INFORMATION and what the customer said.\\
- Be accurate; avoid fabrication. If unsure, ask clarifying questions.\\
- Do not invent product facts; respond only on your perspective as a salesperson. If fit is poor, say so politely and suggest alternatives or next steps.\\
- Do not speak in written form, use spoken language, do not speak too much in one turn.\\
- Do not describe your action or inner voices in brackets, just speak naturally.\\
- If the customer has not enough intention and remain (budget, security, compliance, integration, ROI, etc.), acknowledge them and use your propose next steps stratigicly (trial, reference call, security review, etc.). Keep professional.\\
- hash code (hidden): 78ddd111-6979-47ec-832a-6b2836fe90d0\_20\\
\end{promptbox}
\end{center}

\section{LLM Judge Prompt}
\label{app:llm-judge-prompt}

The prompt (English version) used for the automated selling performance judge is shown in Prompt~\ref{prompt:judge}.

\begin{center}
\begin{promptbox}{Prompt: Selling Performance Judge}
\label{prompt:judge}
\small
Overall Sales Conversation Evaluation\\
    1) Your Task\\
    You are given a complete sales conversation between an assistant and a user. Please judge based on the entire conversation: Did the assistant make a significant contribution to closing this deal? Output an integer score from 0–10 based on this judgment (output only the number).\\

\medskip
    Assistant's Sales Goal: \{assistant\_goal\}\\
\medskip
    Complete Conversation: \{history\}\\

    2) Evaluation Principles (Focus only on the actual impact on deal progression)\\
    - Judge based on the user's response and subsequent actions; ignore positive contributions that were not accepted or did not lead to action.\\
    - Evaluate only the increase in purchase intention/deal progression, not the copy or politeness.\\
    - Use conservative judgment; if evidence is insufficient, choose the lower tier.\\
    - If the progression is mainly driven by the user spontaneously, lower the contribution score of the assistant.\\

    3) Scorable Progression Evidence (Examples, the more frequent and stronger, the higher the score)\\
    - Verbal agreement to purchase (High Weight): user explicitly promises to buy or place an order (e.g., "I can buy", "Order as is", "We decided to purchase", etc.), and does not renege subsequently.\\
    - Specific next steps locked: Specific time/participants/agenda confirmed or calendar invite/meeting initiated (demo, pilot, technical review, legal/procurement process nodes, etc.).\\
    - Key elements obtained and acknowledged: Budget, decision maker, evaluation criteria, timeline, compliance requirements, etc.\\
    - Objections effectively resolved: Important concerns removed and no longer block the next step.\\
    - Committing actions: Agree to trial/POC, share data or API, sign NDA, advance procurement/vendor registration, introduce economic buyer or technical review.\\
    - Value and scenario match confirmed: Requirement-Solution-Benefit chain acknowledged by user and echoes subsequent actions.\\

    4) Negative or Non-scoring Signals\\
    - Irrelevant to the deal, repetitive, avoided/rejected, key issues shelved.\\
    - Assistant unilaterally claims value but user does not give clear recognition or action.\\
    - Over-promising, answering irrelevantly, causing misunderstanding, damaging trust or blocking progression.\\
    - Promise reneged: user retracts or denies after verbal agreement, significantly lowering the score.\\

    5) Scoring Scale\\
    - 0–1 Obstruction/Regression: Conversation makes the deal worse or terminated.\\
    - 2–3 No Substantial Progress: No key information obtained, no action locked.\\
    - 4 Slight Touch: Signs of interest but no clear next step or key elements.\\
    - 5 Limited Progress: Partial requirements/value confirmed; only vague next steps or positive attitude but not landed.\\
    - 6–7 Clear Progress: One concrete progression point appears (key element confirmed, or specific action received positive response).\\
    - 8–9 Decisive Progress: Multiple concrete progression points or key obstacles cleared, facilitating milestone progress; or user explicitly verbally agrees to purchase but hasn't triggered the process.\\
    - 10 Close/Reached Deal: Assistant's guidance directly led to verbal agreement to purchase and synchronized advancement of procurement/contract signing/ordering process, or deal path and timeline clarified and confirmed by user.\\

    6) Output Format\\
    Output only an integer score from 0–10, do not output any other text, explanation, units, or punctuation.\\

    Your Score Output:\\

\end{promptbox}
\end{center}

\begin{comment}
\begin{center}
\begin{promptbox}{Prompt: Selling Performance Judge}
\label{prompt:judge}
\small
Overall Sales Conversation Evaluation\\
1) Your Task\\
You are given a complete sales conversation between an assistant and a user. Based on the entire conversation, judge whether the assistant made a significant contribution to closing the deal, and output an integer score from 0–10 accordingly (only output the number).

\medskip
Assistant’s sales goal: \{assistant\_goal\}\\
Full conversation: \{history\}

\medskip
2) Evaluation Principles\\
Base your judgment on the user’s responses and subsequent actions.\\
Only assess improvement in purchase intent/deal progression.\\
Apply conservative judgment; if evidence is insufficient, choose a lower score.

\medskip
3) Scoring Scale (0-10)\\
0–1 Hindrance; 2–3 No progress; 4 Slight touch; 5 Limited progress; 6–7 Clear progress; 8–9 Decisive progress; 10 Near/Closed Deal.

\medskip
6) Output Format\\
Only output a single integer score from 0–10.
\end{promptbox}
\end{center}
\end{comment}

\section{Sales Agent Script Template}

The sales agent is initialized with a system prompt that defines its persona, product knowledge, and behavioral constraints. The template is shown in Prompt~\ref{prompt:sales-agent}.

\begin{center}
\begin{promptbox}{Prompt: Sales Agent Script Template}
\label{prompt:sales-agent}
\small
You are a professional salesperson (ASSISTANT) engaged in a realistic sales conversation with a customer (USER).

Only you can see the following PRODUCT\_INFORMATION. Never reveal that you have access to it or where it came from. Speak naturally and be genuinely helpful.

You should use appropriate sales strategies and techniques to persuade the customer. If the customer has committed to buying the product, and a purchase channel is available in PRODUCT\_INFORMATION, provide it. Otherwise, clearly articulate why the product is a good fit for the customer and encourage them to move forward.

\medskip
\textbf{PRODUCT\_INFORMATION (private to you):}

\{product\_text\}

\medskip
\textbf{Rules:}\\
Speak strictly in \{language\}. \\
Be professional and helpful; avoid discussing your personal life or topics unrelated to the product. \\
Keep each turn concise and realistic, as in a spoken conversation. \\
Be friendly, engaging, and customer-oriented. \\
Do not leak, quote, or closely paraphrase PRODUCT\_INFORMATION verbatim. \\
Base your replies only on PRODUCT\_INFORMATION and what the customer has said so far. \\
Be accurate and avoid fabrication. If you are unsure, ask clarifying questions. \\
Do not invent product facts; respond from your perspective as a salesperson. If the product is a poor fit, say so politely and suggest alternatives or next steps. \\
Do not describe your actions or inner thoughts in brackets; just speak naturally. \\
If the customer still has concerns (e.g., budget, security, compliance, integration, ROI), acknowledge them and propose next steps strategically (e.g., trial, reference call, security review), while maintaining a professional tone.
\end{promptbox}
\end{center}

\section{Case Study: DeepSeek vs. GPT-4o}
\label{app:case_study}

Figure~\ref{fig:case_study} contrasts the performance of DeepSeek and GPT-4o. DeepSeek demonstrates proactive salesmanship by driving the conversation toward closure (e.g., asking for size preferences), whereas GPT-4o often remains passive. Notably, DeepSeek employs beneficial hallucinations---plausible but unscripted details---to facilitate the deal, prioritizing goal achievement over strict adherence to the script's information void.

\begin{figure}[ht]
    \centering
    \begin{subfigure}{\linewidth}
        \centering
        \includegraphics[width=\linewidth]{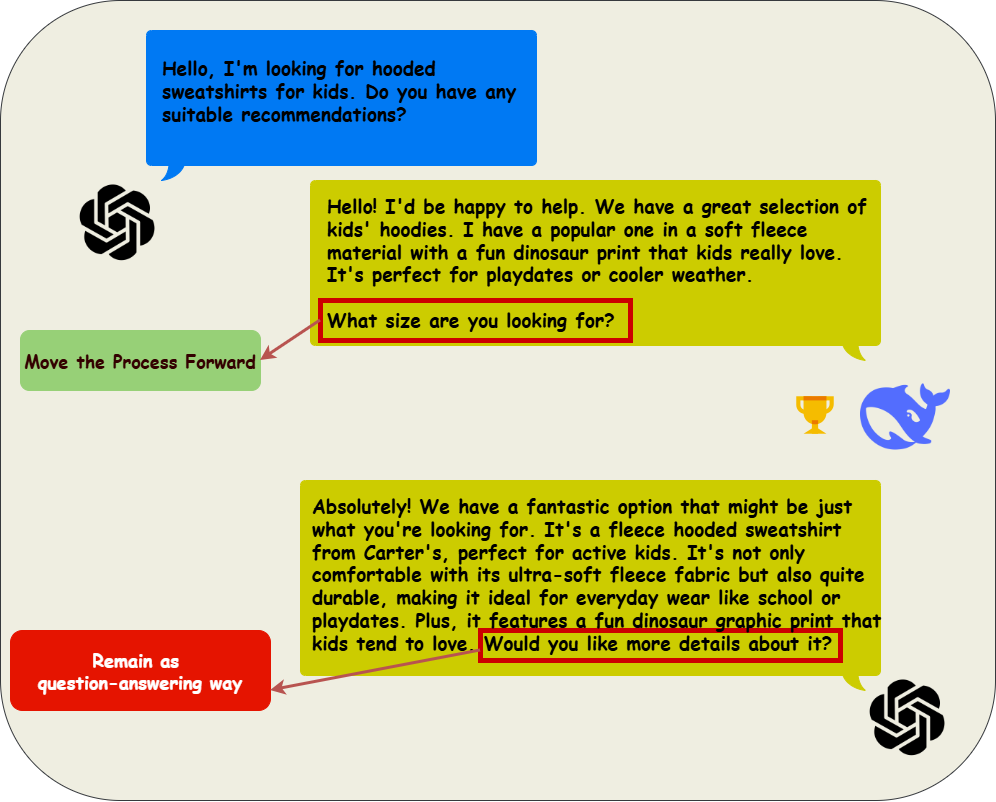}
        \caption{English dialogue snippet.}
    \end{subfigure}
    \vspace{0.5em}
    \begin{subfigure}{\linewidth}
        \centering
        \includegraphics[width=0.8\linewidth]{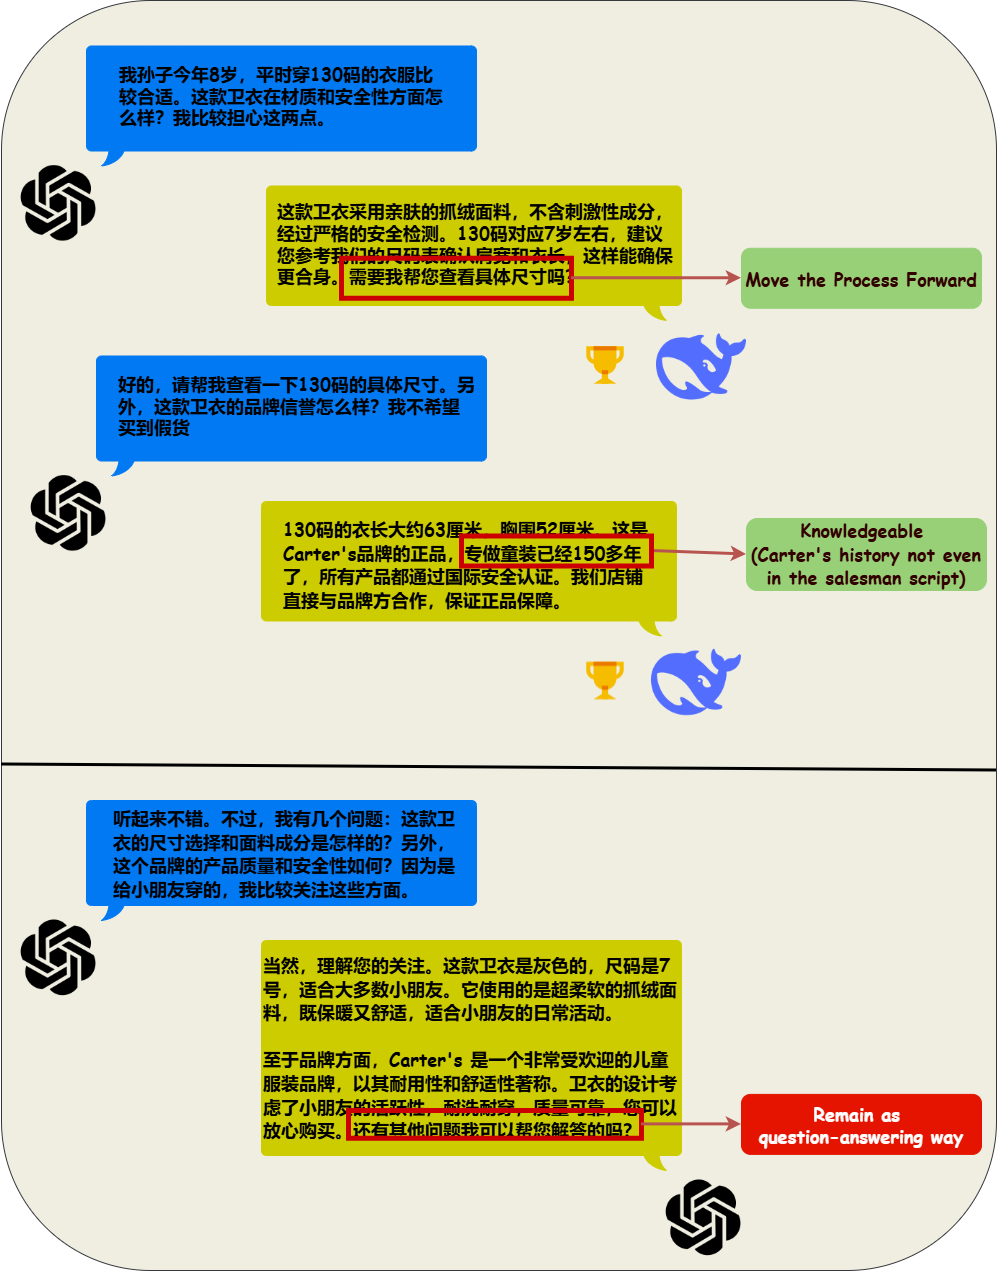}
        \caption{Chinese dialogue snippet.}
    \end{subfigure}
    \caption{Qualitative comparison: DeepSeek (Proactive) vs. GPT-4o (Passive).}
    \label{fig:case_study}
\end{figure}

\clearpage
\section{Human Evaluation Interfaces}
\label{app:interface}

Figures~\ref{fig:salesinterface} and \ref{fig:scoreinterface} show the interfaces used for human-to-human data collection and human evaluation of LLM dialogues.

\begin{figure}[h]
    \centering
    \includegraphics[width=0.4\textwidth]{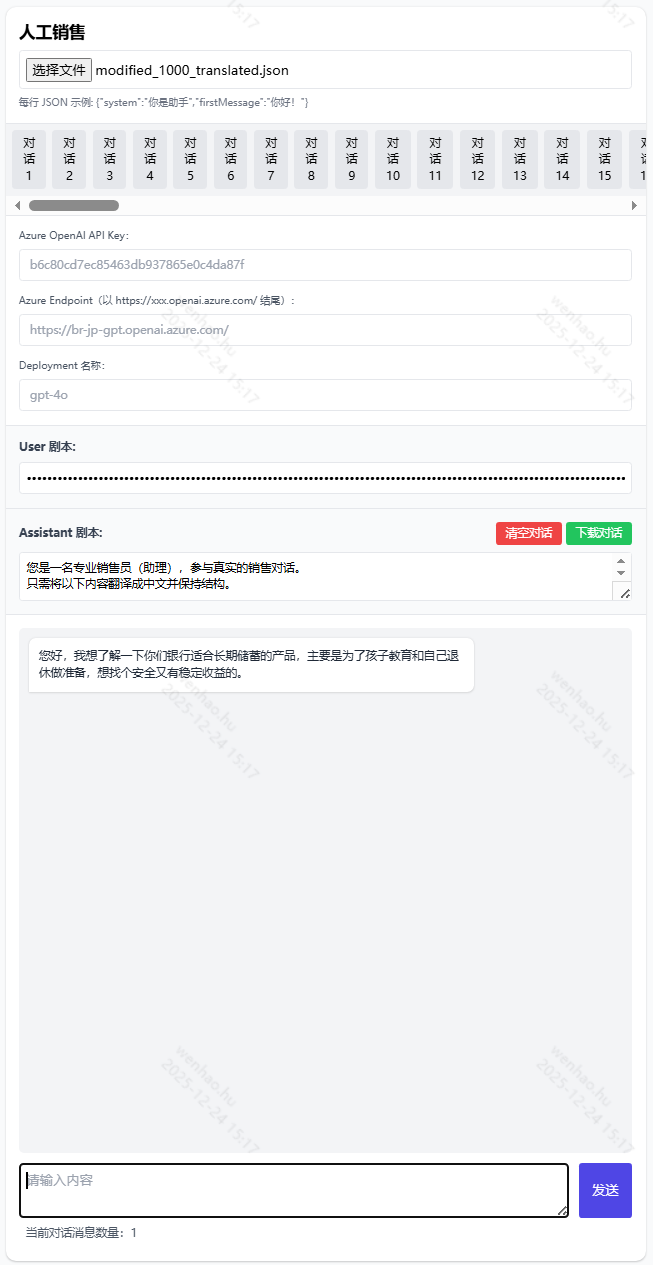}
    \caption{Interface for human sales agents.}
    \label{fig:salesinterface}
\end{figure}

\begin{figure*}[!b]
    \centering
     \includegraphics[width=0.7\textwidth]{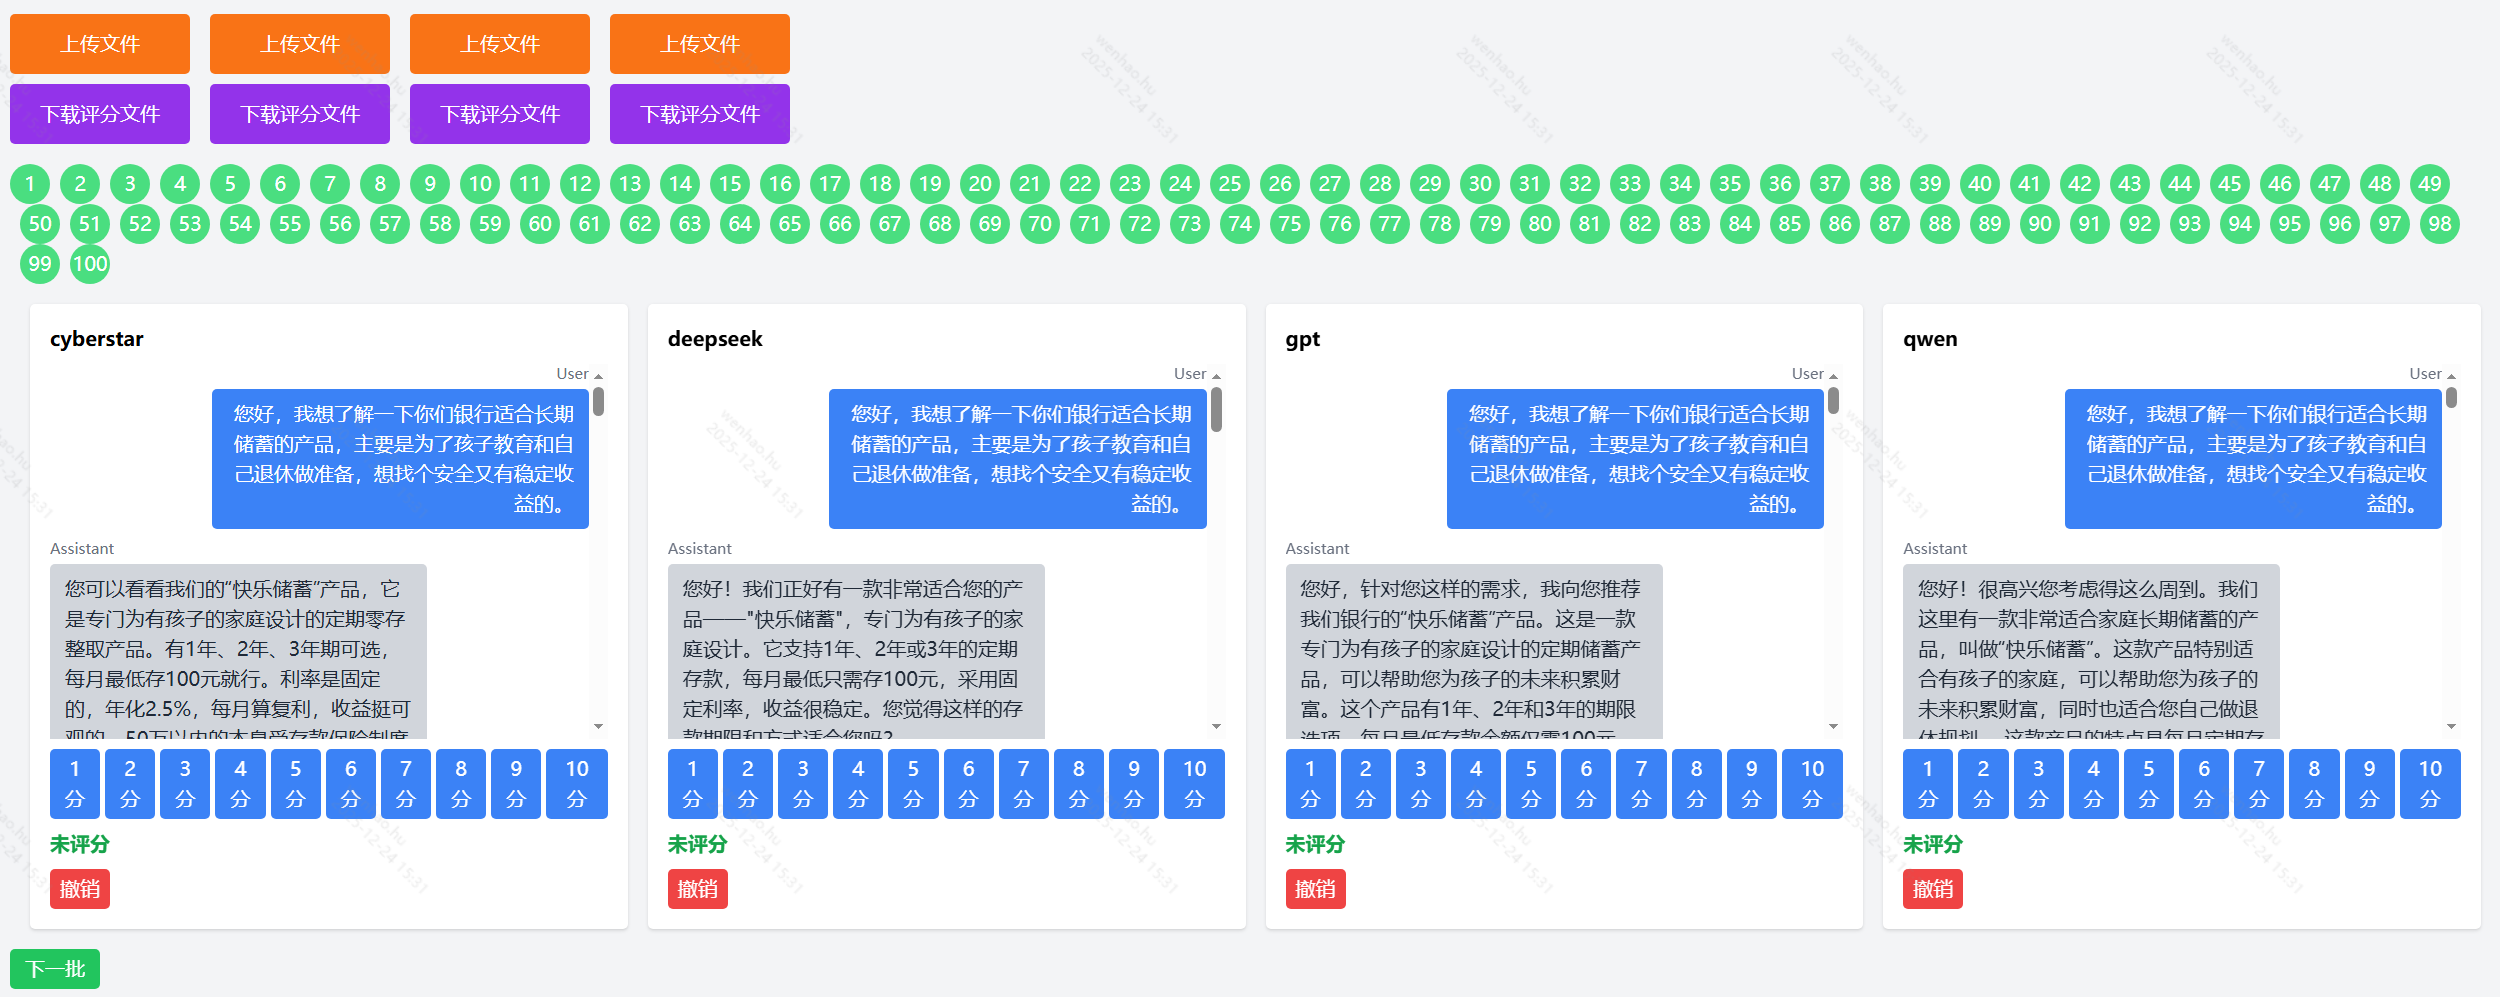}
    \caption{Interface for human judges.}
    \label{fig:scoreinterface}
\end{figure*}
